# Supplementary material for: Faceting and flattening of emulsion droplets: a mechanical model
Source: arXiv:2009.01218 ancillary file (2021-08-02)
Supplement: Supplementary file 1 [file SupplementaryMaterial_GarciaAguilar_2020.pdf]

# Supplementary Material for "Faceting and flattening of emulsion droplets: a mechanical model"

Ireth García-Aguilar,[1] Piermarco Fonda,[1,2] Eli Sloutskin,[3] and Luca Giomi[1]

[1] *Instituut-Lorentz, Universiteit Leiden, P.O. Box 9506, 2300 RA Leiden, Netherlands*
[2] *Theory & Bio-Systems, Max Planck Institute of Colloids and Interfaces, Am Mühlenberg 1, 14476 Potsdam, Germany*
[3] *Physics Department and Institute of Nanotechnology and Advanced Materials, Bar-Ilan University, Ramat Gan 529002, Israel*

(Dated: Monday 2nd August, 2021)

This supplementary information contains details about the computation of the geometry-dependent terms of the energy in Table I of the main text, the model fit shown in Fig. 1f of the main text, and the assumptions relating the energy coupling parameters.

## DROPLET GEOMETRIES

The dimensionless energy $\mathcal{E}$ is obtained from the numerical integration of the mechanical energy Eq. (1) on a triangular discretization of the surface for each of the three droplet shapes studied (see Fig. 1e in the main text). To make the total energy dimensionless, the various contributions are normalized as follows:

$$\mathcal{E}_W = 2\int \mathrm{d}A\, H^2 \,, \quad \mathcal{E}_H R = 4\int \mathrm{d}A\, H \,, \quad \mathcal{E}_S R^2 = \frac{1}{2}\int dA\, \sigma^2 \,, \quad \mathcal{E}_C R^2 = \int dA \,, \quad \mathcal{E}_G R^4 = \frac{1}{2}\int dA\, z^2\, N_z \,.$$

All terms, with the exception of the stretching term $\mathcal{E}_S$ depend solely on the droplet geometry. Details about the calculation of the stretching energy are reported in the following Section. The local mean and Gaussian curvatures are computed from the triangular discretization of the surface as described in Ref. [26].

All triangulated surfaces were constructed using the software Surface Evolver [27]. The rounded icosahedron was obtained from the sharp one with perfectly flat faces, which were refined to have around $2 \times 10^4$ mesh points. Using the software, we allowed an area-minimizing relaxation of the icosahedron into a sphere. The icosahedral shape used for this study is an intermediate stage of the relaxation with rounded edges and vertices of finite curvature, while the sphere is the final shape (see Ref. [25] for more details). Similarly, the hexagonal platelet was initialized as a perfectly sharp polyhedron with $\approx 2 \times 10^4$ mesh points and its edges and vertices were rounded with a smoother relaxation and further regularization. The rounded edges of the icosahedron and the platelet have on average an approximate mean curvature of $\bar{H}^2_{\rm ico} R^2 = 3.2$ and $\bar{H}^2_{\rm pla} R^2 = 21.9$ respectively, in contrast to that of the sphere $\bar{H}^2_{\rm sp} R^2 = 1$.

The height of the resulting platelet, measured along the direction of gravity is 7% the width of the hexagonal face, consistent with scanning electron microscopy of these droplets [23]. See for example in Fig. S1 a 3D cross-section of a hexagonal platelet.

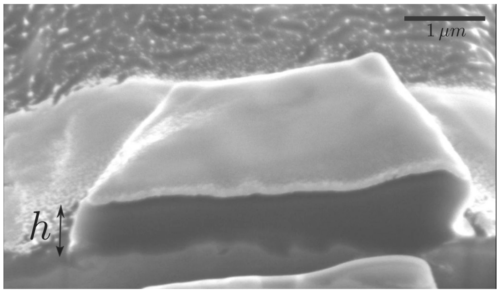


Fig. S1: Focused Ion Beam (FIB) slicing through a polymerized hexagonal platelet, evincing the approximate height-to-width ratio in these droplets to be of the order of 1 : 10. Taken and modified with permission from the Supplementary Information in Ref. [23].

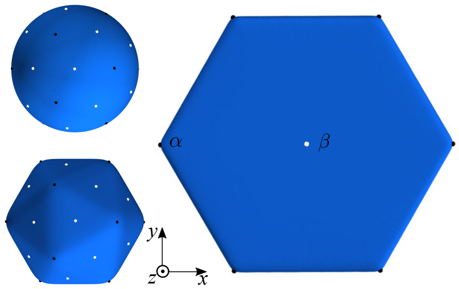


Fig. S2: Modeled droplet shapes for the calculation of the energy, viewed along the direction of gravity. These are to scale according to a fixed size $R$. Each surface is marked with the positions of the “seed” disclinations $\boldsymbol{r}_\alpha$ (black) and the terminating positions of the dislocation flux $\boldsymbol{r}_\beta$ (white) assumed in the calculation of Eq. (4). The markers have been magnified and do not reflect the underlying discretization of the surface.

## STRETCHING ENERGY

As outlined in the main text, the stretching energy $E_S = Y/2 \int dA\, \sigma^2$, where $Y$ is the Young's modulus, requires finding the stress field $\sigma$ by solving the equation

$$\nabla^2 \sigma = \eta - K \, , \tag{S1}$$

where $\nabla^2$ is the Laplace-Beltrami operator, $K$ is the Gaussian curvature and $\eta$ is the topological charge density of the defects, and it therefore depends on the specific lattice structure of the frozen interface of the droplets. More specifically, it depends on the number, charge and position of the lattice defects. Given the nanoscopic nature of the surfactant-alkane structure at the interface, and the microscopic scale of the droplets themselves, the crystalline monolayer is expected to have a high density of lattice sites. We therefore take the continuous approach described in Ref. [25] for dense crystals, which takes into account possible screening of dislocation structures in the vicinity of the topological disclinations. Within this framework, $\eta$ can be expressed in terms of the topological charge density of twelve topologically required disclinations plus the effective charge density resulting from a continuous distribution of screening dislocations, i.e. Eq. (4) in the main text. The latter is described by two sets of discrete defects with different charge: defects screening out the disclination-induced stress in the vicinity of the disclination positions $\boldsymbol{r}_\alpha$, and additional defects located close to the far end of these dislocation structures, in positions $\boldsymbol{r}_\beta$.

As explained in Ref. [25], the resulting stretching energy is found to have a quadratic scaling with the droplet size and can be expressed as

$$E_S = Y \mathcal{E}_S R^2 = \frac{Y}{2} \left[ c_0 - \frac{c_1^2}{4 c_2} \right] R^2 \, , \tag{S2}$$

where the coefficients depend on the particular surface geometry and the distribution of defects for the charge density $\eta$ in Eq. (4). For more details on this calculation we refer the reader to Ref. [25]. In particular, we use here the coefficients calculated in this reference for the sphere and the rounded icosahedron. We show these and the resulting coefficients for the platelet in Table SI. Finally, we note that in the case of little to no screening, $\Phi = 0$ in Eq. (4), the coefficients $c_1 = 0$ and $c_2$=0, therefore equivalent to a rescaling of the coupling parameter $Y$ (and hence $\Gamma$), which is different for every shape.

## MODEL FIT TO EXPERIMENTAL DATA ON SIZE-DEPENDENCE OF THE TRANSITIONS

The experimental data shown in Fig. 1f of the main text were taken with permission from Fig. S4 in Ref. [3], used in this work with slightly improved statistics (see text Ref. [3] for more details). In these experiments, droplets of various initial sizes are imaged at slow cooling, in order to identify the temperature at which the individual droplets first facet and further flatten and measure the surface tension then. Given the scatter in the measurements for different droplets, it is convenient to take the difference between the surface tension at the sphere-icosahedron

| Shape | $c_0$ | $c_1$ | $c_2$ |
|---|---|---|---|
| Sphere | 0.046 | -0.12 | 0.093 |
| Icosahedron | 0.0061 | -0.039 | 0.11 |
| Platelet | 0.0032 | -0.042 | 8.2 |

Table SI: Coefficients of the stretching energy, Eq. (S2), for the spherical, icosahedral and hexagonal geometries, calculated using the framework described in Ref. [25].

transition $\gamma_{\rm sph-ico}$ and the icosahedron-platelet transition $\gamma_{\rm ico-pla}$, denoted as $\Delta\gamma(R)$, where $R$ is the radius of the spherical droplet before faceting. We consider the results for droplets of sizes in the range $R = 2.2 - 133\,\mu$m, and further bin these data to reduce dispersion. The value of the surface tension $\gamma$ is estimated under the assumption that this is the only material parameter significantly affected by temperature within the experimental range [3]. This is justified by the fact that the bulk modulus is related, through the Grüneisen constant, to the heat capacity and the thermal expansion [28]. The thermal expansion for similar interfacial crystals was measured to be temperature-independent in the relevant range of temperatures [29]. Moreover, since $dS/dT$ of the interfacial crystal is constant, up to its melting point [4], the temperature-variation of the heat capacity $C = T(dS/dT)$ should be $\sim 0.3\%/^\circ C$. Thus, the bulk modulus does not significantly change in the relevant range of temperatures. Similar arguments allow the assumed temperature-independence of the other moduli to be justified [30].

We obtain the model prediction for $\Delta\gamma(R)$ starting from the energy functional proposed in Eq. (3) of the main text. Using the dimensionless energy terms introduced above in this supplementary information and whose values can be found in Table SI for the three shapes studied, we can write the energy as

$$E = \kappa\mathcal{E}_W - \kappa H_0 \mathcal{E}_H R + (\gamma\mathcal{E}_C + Y\mathcal{E}_S)R^2 + g\Delta\rho\mathcal{E}_G R^4 \,, \tag{S3}$$

in terms of the material constants $\kappa$, $\gamma$, $Y$, and the density difference between the oil and water. We solve the equations $E_{\rm sph} = E_{\rm ico}$ and $E_{\rm ico} = E_{\rm pla}$ to find the critical surface tension as a function of size $\gamma(R)$, at the faceting and the flattening respectively. We can then compare the experimental measurements to the model prediction for $\Delta\gamma = \gamma_{\rm sph-ico} - \gamma_{\rm ico-pla}$. Taking $\Delta\rho = 0.25\,{\rm g/cm}^3$ [4, 11] and $\kappa = 10^3 k_B T$ [3], we fit $\Delta\gamma(R)$ to the experimental measurements, considering $Y$ and $H_0$ as free fitting parameters. Using non-linear least squares fitting, we find the solid red curve shown in Fig. 1f, for which $H_0^{-1} \approx 58,{\rm nm}$, and $Y \approx 4.4\,{\rm mN/m}$. For an interface of thickness 2 nm [3], this roughly corresponds to a 3D Young's modulus of $Y_{\rm 3D} = 2\,{\rm MPa}$.

The dimensionless parameters used in the morphological phase diagram in Fig. 2 were estimated considering the values of the material constants resulting from the fit. In particular, we adopt $\Upsilon = 4$ and $\Pi \approx 10^{-8}$. Note that a small variation in $\gamma$, such as those reported in Ref. [4], would not change the results, provided that the dimensionless values of $\Upsilon$, $\Gamma$ and $\Pi$ are kept the same, which can be achieved by a small variation of $\kappa$, $H_0$ and $Y$.

## ENERGY CONTRIBUTIONS AT DIFFERENT SCALES

In Table SII, we report the magnitude of the dimensionless energy differences, $\Delta\mathcal{E} = \mathcal{E}_{\rm ico} - \mathcal{E}_{\rm sph} = 0$, appearing in the main text, at different size scales. Since each energy term scales differently with $r$, their relative magnitude varies with the droplet size. At the smallest sizes, it is the bending term, including the spontaneous curvature, which plays a leading role in the observed size-dependent behavior of the faceting. For droplets of $r \approx 10^2$, we find that elasticity competes with the surface tension, while buoyancy is the main deforming component at the large scale. A similar analysis holds for the flattening. In this second transition, the stronger influence of gravity is reflected quantitatively in a larger $\Delta\mathcal{E}_G$

| | $\lvert\Delta\mathcal{E}_W\rvert$ | $\lvert\Delta\mathcal{E}_H\rvert\ r$ | $\lvert\Gamma\Delta\mathcal{E}_C + \Upsilon\Delta\mathcal{E}_S\rvert\ r^2$ | $\Pi\lvert\Delta\mathcal{E}_G\rvert\ r^4$ | Leading term |
|---|---|---|---|---|---|
| $r \approx 10$ | 24 | 6 | 2 | $2 \times 10^{-4}$ | Bending |
| $r \approx 10^2$ | 24 | 60 | 200 | 2 | Stretching |
| $r \approx 10^3$ | 24 | 600 | $2 \times 10^4$ | $2 \times 10^4$ | Gravitational |

Table SII: Estimate of the energy contributions at different scales during faceting. The transition is determined by the difference in the dimensionless energy, Eq. (3), between a spherical droplet and an icosahedral one, $\Delta\mathcal{E}$. The dimensionless material parameters here are taken as $\Gamma = 0.1$, $\Upsilon = 4$ and $\Pi = 10^{-8}$.
